# Supplementary material for: When Lipschitz Walks Your Dog: Algorithm Engineering of the Discrete Fr\'echet Distance under Translation
Source: arXiv:2008.07510 source file (2020-08-17)
Supplement: Supplementary file 1 [file preliminaries_appendix.tex]

\section{Useful Properties of the Fréchet Distance Under Translation}
\label{sec:prelim_appendix}
